# Supplementary material for: Making Quantum Local Verifiers Simulable with Potential Applications to Zero-Knowledge
Source: arXiv:2209.10798 source file (2022-09-22)
Supplement: Supplementary file 1 [file appendix.tex]

\section{Hardness of Approximate $\CLDM$}

The Consistency of Local Density Matrices ($\CLDM$) problem is known to be $\QMA$-complete under Karp-reduction~\cite{BroadbentG20}. Previously, it was proved by Liu~\cite{Liu06} to be $\QMA$-complete under Turing-reduction.	The problem statement is very simple: 

\begin{definition}[$\CLDM$] Let $k \in \N$ be a constant.	Given $m$ $k$-local constraints on $n$ qubit (mixed) $\sigma$ such that the $i$-th constraint requires $\Tr_{[n] \setminus S_i}[\sigma] = \rho_i$. The task is to determine between (1) there exists such an $\sigma$ satisfying all $m$ constraints and (2) for all $n$-bit quantum state $\sigma$, there exists at least $i \in [m]$ such that
	\[
	\| \sigma_{S_i} - \rho_i \|_{\tr} \ge \gamma(m),
	\]
	where $\gamma$ is a polynomial in $m$.
\end{definition}

Inspired by the $\QPCP$ conjecture, we hope to consider the gapped version of $(\alpha,\beta,\gamma)\text{-}\gapCLDM$, defined as follows:

\begin{definition}[$(\alpha,\beta,\gamma)\text{-}\gapCLDM$]
	Let $k \in \N$ be a constant, and $0 < \beta <\alpha \le 1$ be two constants. Given $m$ $k$-local constraints on $n$ qubit (mixed) $\sigma$ such that the $i$-th constraint states $\Tr_{[n] \setminus S_i}[\sigma] = \rho_i$, and the task is to determine between (1) there exists such an $\sigma$ satisfying at least $\alpha\cdot m$ constraints and (2) for all $n$-bit quantum state $\sigma$, there are at most $\beta m$ such that
	\[
	\| \sigma_{S_i} - \rho_i \|_{\tr} > 1/\gamma(m),
	\]
	where $\gamma$ is a function from $\N$ to $\R$.
\end{definition}

%We will first study the $\QMA$-hardness of $(\alpha,\beta,m^{-c})\text{-}\gapCLDM$ for a big constant $c$.

%\cljnote{There is some issue in generalizing this further to $\gamma(m)$ being constant. Need to understand~\cite{bausch2018analysis} better to resolve this I think...}

We are interested in the hardness of approximate $\CLDM$.

\begin{question}
	Is $\QMA$-hardness of $\gapCLDM$ for some constants $\alpha,\beta,\gamma$ equivalent to $\QPCP$ (under Karp reduction)?
\end{question}

We have the following two results.

\begin{theorem}[Easy direction]
	If for some constants $0 < \beta<\aleph \le 1$ and $\gamma > 1$, $(\alpha,\beta,\gamma)\text{-}\gapCLDM$ is $\QMA$-hard, then $\QPCP$ holds.
\end{theorem}

%The other direction seems more difficult, but I speculate that the techniques from~\cite{BroadbentG20} combined with space-time Hamiltonian construction may imply it. \cljnote{TODO: work the details out}

Applying the techniques from~\cite{BroadbentG20}, we can show a partial result regarding the other direction.

\begin{theorem}
	$\QPCP$ implies that for some constants $0 < \beta< \alpha \le 1$ and $c \ge 1$, $(\alpha,\beta,m^{-c})\text{-}\gapCLDM$ is $\QMA$-hard.
\end{theorem}

\section{A variant of $\NLTS$} 

Suppose $\gapCLDM$ is $\QMA$-complete. Then it should not be in $\NP$. This should imply a variant of $\NLTS$ with respect to $\gapCLDM$.

It is not hard to give $m$ local constraints on $n$ qubits. Such that for a small constant $c_0 > 0$, for any state $\sigma$ such that $\| \sigma_{S_i} - \rho_i \|_{\tr} \le c_0$ for at least $(1-c_0)$ fraction of $i$ from $[m]$, we have $\cc(\sigma) \ge \Omega(\log n)$.

The construction is very simple: take an expander graph on vertex set $[n]$, for each edge $(u,v)$, we add a constraint
\[
\left\| \sigma_{\{u,v\}} - \frac{1}{2}(\spz{0}\rpz{0} + \spz{1}\rpz{1}) \right\|_{\tr} \le 10^{-9}.
\]

\begin{proofsketch}
	Let $G = ([n],E)$. We first delete the $(1-c_0)$ fraction of edges which are violated to obtain an edge set $E'$.
	
	Next, consider the random variable $\bX$ obtained by measuring $\sigma$ in the computational basis. We know that in expectation $\bX$ satisfies $(1-10^{-9})$ fraction of edges in $E'$. This further implies in expectation $\bX$ violates a $c_0 + 10^{-9}$ fraction of edges in $E$, meaning that with probability at least $0.99$, $\bX$ has at least $1-O(c_0 + 10^{-9})$ fraction of $1$'s or $0$'s.
	
	Finally, note that $\Ex[\bX_i] = 1/2$ for all endpoints in $E'$, meaning that $\Ex[|\bX|]$ is close to $n/2$. Hence one can show the distribution of $\bX$ is $(\Omega(1),\Omega(n))$-separable, and thereby an $\Omega(\log n)$ lower bound follows from~\cite{EldarH17}.
	
\end{proofsketch}
